# Supplementary material for: Decide: Knowledge-Based Version Incompatibility Detection in Deep Learning Stacks
Source: arXiv:2408.02133 source file (2024-08-04)
Supplement: Supplementary file 1 [file 99-Appendix.tex]

% %%
% %% If your work has an appendix, this is the place to put it.
\appendix

\section{TOOL WALKTHROUGH}

\subsection{Introduction}
Deep learning (DL) models have been widely utilized across various domains. However, complex dependencies among deep learning components often cause challenging version incompatibility issues. Moreover, these version incompatibility issues are always hard to detect and resolve.

\webtool{} is an interactive knowledge-based tool for detecting and identifying version (in)compatibility in deep learning stacks. Specifically, \webtool{} allows users to gain a comprehensive understanding of the (in)compatibility relations between deep learning components through knowledge graph visualization, search query, and detailed post exploration. In this appendix, we provide a detailed walkthrough of the tool, highlighting its key features and functionalities.

\subsection{Setup and Requirements}
We have made \webtool{} public at \url{https://github.com/LexieZhou/Decide}. Here are the steps to set up \webtool{}.
\begin{itemize}
\item Install \texttt{Node.js} for your operating system~\footnote{The latest version and installation instruction can be found at \url{https://nodejs.org}.}
  \item Clone or download the repository
  \begin{itemize}
    \item \texttt{git clone https://github.com/LexieZhou/Decide.git}
  \end{itemize}
  \item Install dependencies
  \begin{itemize}
    \item Direct to server directory and call \texttt{npm install}.
    \item Direct to client directory and call \texttt{npm install}.
  \end{itemize}
  \item Start the Project
  \begin{itemize}
    \item Direct to server directory and call \texttt{node server.js}.
    \item Direct to client directory and call \texttt{npm start}.
  \end{itemize}
\end{itemize}

\subsection{Demonstration Steps}
After setting up \webtool{}, users will access the landing page of \webtool{} and find a knowledge graph containing 2,376 version knowledge extracted from Stack Overflow discussions.

\subsubsection{The Compatibility Visualizer}
The Compatibility Visualizer (Figure~\ref{fig:overview} A) allows users to interact with the knowledge graph. Users can zoom in, zoom out, and drag to explore the details of the graph. Each node within the knowledge graph represents a versioned deep learning stack component. Next to each node, \webtool{} displays the component name and version. The color of the nodes indicates their belonging to a specific stack layer. When hovering over a node, users can view detailed information about the component in the right corner of \webtool{}. 

The links between nodes represent their (in)compatibility relationships. Solid links indicate compatibility, while dashed links indicate an incompatibility relationship between two components. The predicted (in)compatibility relationship is determined based on the number of posts supporting compatible and incompatible relationships.

\subsubsection{The Information Panel}
The Information Panel (Figure~\ref{fig:overview} B) provides two types of representations. When a specific deep learning library is clicked, the panel presents detailed information about the library sourced from \textit{Libraries.io}. This information includes keywords, licenses, dependencies, and release times. Users can also click on the statistics in the information panel to seamlessly navigate to the repository page of the DL component library, where they can access more detailed information.

When a link between two components is clicked, the information panel displays details about the two components, their detected (in)compatibility relationship, a confidence score, and supporting posts. For a pair of versioned components, let $\#\textit{Compatible}$ represent the number of posts \webtool{} infers a compatible relationship between them, and $\#\textit{Incompatible}$ denote the number of posts that \webtool{} infers an incompatible relationship. We define the confidence score of the relationship between two versioned components as follows: $\textit{confidence score} = \frac{{\#\textit{Compatible} - \#\textit{Incompatible}}}{{\#\textit{Compatible} + \#\textit{Incompatible}}}$. If \textit{confidence score} is a positive number, it implies a compatible relationship. Otherwise, it implies an incompatible relationship. Relationships with a neural confidence score are discarded. Additionally, users can explore posts supporting both compatible and incompatible relationships. The posts are ranked by votes by default, and clicking on the vote link takes users directly to the original posts on the Stack Overflow platform. This feature makes it easy to find relevant solutions for version incompatibility issues.

\subsubsection{Search Bar}
The search query (Figure~\ref{fig:overview} C) is a standout feature of \webtool{}. It supports three types of searches. First, users can quickly check the compatibility between two deep learning components by entering a simple query. For example, users can ask, "Does \texttt{Python 3.6.8} work with \texttt{Ubuntu 16.04.6}?" The tool will display the \texttt{Python 3.6} and \texttt{Ubuntu 16.04} nodes, along with their relationship. Users can then click the link to explore further details.

Second, users can search for compatible components for a specific version to view all the relationship knowledge associated with that component. For example, searching for \texttt{Ubuntu 14.04} will display \texttt{Ubuntu 14.04}, all its connected deep learning components, and their corresponding (in)compatible relationships.

Lastly, users can explore a deep learning stack component without specifying a version. \webtool{} will display all versions of that component and their compatibility relationship knowledge. For instance, searching for \texttt{Tensorflow} will show all versions and their connected deep learning components. If users input DL components that do not exist in the knowledge graph, \webtool{} will issue an alert, suggesting users explore other potential resources.

\subsubsection{The Statistical Panel}
The left panel (Figure~\ref{fig:overview} D) of \webtool{} displays statistical information about the top entities in each deep learning layer, including driver, library, application, operating system, and runtime. Each bar chart showcases the top five deep learning components with the most (in)compatibility relations. Hovering over a bar allows users to filter the knowledge graph to display the corresponding deep learning stack component and its compatibility relationships in the Compatibility Visualizer.

\subsection{Conclusion}
\webtool{} provides an interface for users to easily navigate version incompatibility issues, find compatible components, and access relevant solutions based on Stack Overflow discussions. Its powerful features streamline deep learning models and applications reuse.
